# Supplementary material for: Scaling of phloem structure and optimality of photoassimilate transport in conifer needles
Source: arXiv:1412.1272 source file (2014-12-03)
Supplement: Supplementary file 1 [file supplemental_material.pdf]

# Scaling of phloem structure and optimality of nutrient transport in conifer needles – Supplementary Information

Henrik Ronellenfitsch, Johannes Liesche, Kaare H. Jensen, N. Michele Holbrook, Alexander Schulz, Eleni Katifori

July 25, 2014

The phloem in conifer needles typically consists of a bundle of vascular cells called sieve elements long strands of which make up so called sieve tubes. Nutrient transport occurs according to the Münch mechanism; by loading sugars into the sieve elements, an osmotic gradient is established which draws water into the cells, thus establishing a hydrostatic pressure gradient that drives bulk flow. The typical size of sieve elements is roughly constant over the length of the needle. However, their number, and therefore the total area of conductive tissue, increases towards the petiole.

## 1 Numerical analysis of constitutive equations

Nutrient transport in the phloem can be approximately described by the set of equations

$$u(x) = -\frac{k}{\mu}\frac{dp}{dx} \tag{1}$$

$$\frac{dQ}{dx} = 2\frac{L_p A}{r_0}(RT\Delta c - \Delta p) \tag{2}$$

$$\frac{dJ}{dx} = \Gamma \tag{3}$$

Here, $u(x)$ is water flow velocity in the needle, $A(x)$ is total cross sectional area of the vascular bundle, $Q(x) = A(x)u(x)$ the water volume flow, $r_0$ the typical cross-sectional radius of one sieve element, $L_p$ the sieve element membrane permeability, $R$ the universal gas constant, $T$ temperature, $\Delta c = c(x) - \tilde{c}$ the concentration gradient between inside and outside of the sieve

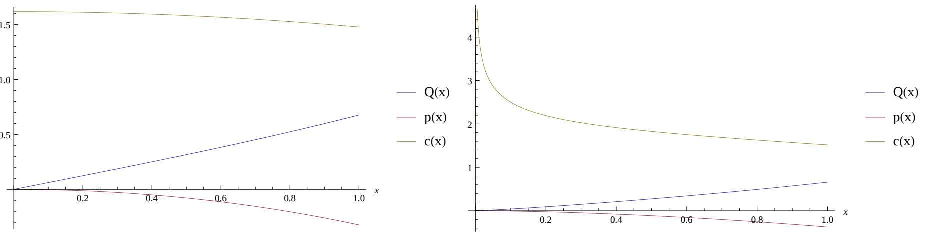


(a) $A(x) = 1, \tilde{\Delta} = -0.5$ (b) $A(x) = \sqrt{x}, \tilde{\Delta} = -0.5$

Figure 1: Numerical solutions of the system of coupled ODEs describing sugar flow for different functions $A(x)$. The $x$ axis corresponds to normalized distance from tip, the $y$ axis is in arbitrary units. We choose to look at (a) $A(x) = 1$, (b) $A(x) = \sqrt{x}$. In case (a), the concentration profile is close to constant, whereas in case (b), there is a singularity at the tip due to the unrealistic condition $A(0) = 0$. In reality, the sieve elements have a finite size such that the approximation breaks down very close to the tip. Still, after roughly 10% needle length, the approximation is applicable and the concentration profile is nearly constant (slightly decreasing). The system of ODEs was solved using Mathematica 9.0.1 (Wolfram Research).

elements, $\Delta p = p(x) - \tilde{p}$ the pressure gradient between inside and outside of the sieve elements, $J(x) = Q(x)c(x)$ total sugar current and $\Gamma$ sugar loading rate. The system can be simplified by solving eqn (3) first, resulting in

$$c(x) = \frac{\Gamma x}{Q(x)}, \tag{4}$$

where we imposed the boundary condition $J(0) = 0$ at the tip of the needle. The simplified system can be written as

$$Q(x) = -\frac{k}{\mu} A(x) \frac{dp}{dx} \tag{5}$$

$$\frac{dQ}{dx} = 2 \frac{L_p A(x)}{r_0} \left( RT \frac{\Gamma x}{Q(x)} - p(x) + \tilde{\Delta} \right), \tag{6}$$

where we absorbed external concentration and pressure into the parameter $\tilde{\Delta} = RT\tilde{c} - \tilde{p}$.

Figure 1 shows the numerical solution of the system for two simple choices of $A(x)$. It should be noted that in principle the continuous approximation breaks down close to the tip of the needle because the effects of discrete sieve elements cannot be neglected anymore. This is reflected

by the appearance of a singularity in the concentration profile at $x = 0$. However, after roughly 10% needle length, both geometries show roughly constant (slightly decreasing) concentration profiles.

# 2 Optimization of nutrient transport

## 2.1 Analytical arguments in the lowest order approximation model

Besides the power dissipation optimization as discussed in the main paper, there are several quantities one can consider relevant for plant fitness. Considerations on whole plant hydraulics have revealed [2] energy flux (or the proportional nutrient flux $j$) as quantities that appear to be optimized for on the level of the whole tree.

On the level of the model described by equations (1,2,3), under the assumption of fixed total conductive volume, $\int_0^L A(x)dx = 1$, one can consider for optimization the fluxes and volume currents

$$J(L) = Q(L)c(L) \tag{7}$$

$$j(L) = \frac{Q(L)c(L)}{A(L)} \tag{8}$$

$$\langle j \rangle = \frac{1}{L}\int_0^L dx j(x) \tag{9}$$

Under the model described above, we find that $J(L) = \Gamma L$, a fixed quantity for fixed needle length. The similar function $j(L)$ can be made arbitrarily large by suitable choice of the function $A(x)$ (which will still satisfy the constraint, for example take $A(x) = \frac{\gamma+1}{L}(x/L)^\gamma$ and let $\gamma \to \infty$). The average nutrient current $\langle j \rangle$ can be optimized by integrating eqn. (3) and employing the method of Lagrange multipliers. The optimum geometry is indeed given by $A(x) \sim x^{1/2}$. However, as can be easily seen by comparing the optimal average current to the one obtained from $A(x) \equiv \text{const}$, this is a local *minimum* of the functional:

$$\frac{\langle j \rangle_{A(x)\sim\sqrt{x}}}{\langle j \rangle_{A(x)\sim\text{const}}} = \frac{8}{9}. \tag{10}$$

The choice of ansatz function $A(x) = \frac{\gamma+1}{L}(x/L)^\gamma$ reveals a singularity at $\gamma = 2$ (fixing $A(0) = 0$).

We must therefore conclude that at the lowest order approximation, energy flux in the needle or out of the needle is not a suitable optimizing

functional, and cannot explain the observed phloem geometry in the needle. On the contrary, the observed needle geometry in fact leads to *minimum* average sugar flux.

## 2.2 A first order loading model

It is possible to consider higher order approximation models for the loading function, effectively modifying eqn (3). One simple generalization is diffusion-like loading which introduces a fixed external sugar concentration $\sigma$ that is used to create an osmotic gradient from the outside of the phloem tissue [1]. The resulting replacement for eqn. (3) is

$$\frac{dJ}{dx} = \beta(\sigma - c(x)), \tag{11}$$

where $\beta$ is an effective diffusion constant for sugar through the lateral membranes, and $\sigma$ the external concentration. The resulting set of equations is studied numerically using a discretization approach. We discretize the real line into nodes $i = 1, 2, \ldots$ and edges $(ij) = (12), (23), \ldots$ with coordinates $x_i = N/i$, where $N$ is the total number of discretization steps. This can be seen as a model of nodes and bonds, where the bonds can be interpreted as short sections of the sieve tubes where the number of sieve elements does not appreciably vary.

Defining the number of tubes at bond $(ij)$ as

$$N_{ij} = \phi \frac{\pi R_{ij}^2}{\pi r_0^2}, \tag{12}$$

where $\phi$ is a covering fraction and $R_{ij}$ is the bundle radius, we find for the constitutive equations (explicitly fixing volume)

$$Q_{ij} = N_{ij} \frac{\pi}{8\mu} \frac{r_0^4}{L_{ij}} (p_j - p_i) \tag{13}$$

$$q_{ij} = N_{ij} 2\pi r_0 L_{ij} L_p (RTc_{ij} - \langle p \rangle_{ij} + \tilde{p}) \tag{14}$$

$$\Gamma_{ij} = \beta(\sigma - c_{ij}) \tag{15}$$

$$V = \sum_{(ij)} N_{ij} \pi r_0^2 L_{ij}, \tag{16}$$

Here, $Q_{ij}$ is the water flow from node $j$ to $i$, $q_{ij}$ the water inflow along bond $(ij)$, $\Gamma_{ij}$ the sugar loading rate along bond $(ij)$, $\mu$ is viscosity, $L_p$ membrane permeability for water, $p_j$ water pressure are node $j$, $\langle p_{ij} \rangle = (p_i + p_j)/2$, $R$ is the universal gas constant and $T$ absolute temperature.

Inserting the expression for $N_{ij}$ and nondimensionalizing using the following scales,

$$Q_c = \frac{2V}{r_0} L_p RT\sigma \tag{17}$$

$$L_c = \left(\frac{r_0^3}{16\mu L_p}\right)^{1/2} \tag{18}$$

$$R_c = \left(\frac{V}{\phi\pi}\right)^{1/2} \left(\frac{16\mu L_p}{r_0^3}\right)^{1/4} \tag{19}$$

$$p_c = RT\sigma \tag{20}$$

$$c_c = \sigma, \tag{21}$$

we obtain the following set of nondimensional equations.

$$Q_{ij} = \frac{R_{ij}^2}{L_{ij}}(p_j - p_i) \tag{22}$$

$$\sum_j Q_{ij} + \frac{1}{2}\sum_j q_{ij} = 0 \tag{23}$$

$$\sum_j Q_{ij} c_{ij} + \frac{1}{2}\sum_j \Gamma_{ij} = 0 \tag{24}$$

$$q_{ij} = L_{ij} R_{ij}^2 (c_{ij} - p_{ij} + \Delta) \tag{25}$$

$$\Gamma_{ij} = \zeta(1 - c_{ij}) \tag{26}$$

$$1 = \sum_{(ij)} R_{ij}^2 L_{ij}, \tag{27}$$

where we introduced $\Delta = \tilde{p}/RT\sigma$ and $\zeta = (\beta/\alpha RT\sigma)(r_0/2V)$.

The set of discrete equations (22–26) can be solved for given $R_{ij}^2$ by transforming into a set of linear equations involving the Laplacian matrix, by plugging eqn. (22) into the continuity equation for water (23). When optimizing, eqn. (24) is enforced as a set of constraints in addition to eqn. (27).

The optimization function we consider is given by

$$J_0 = Q_{01} c_{01} + \frac{1}{2}\Gamma_{01}. \tag{28}$$

This corresponds to the total sugar volume flow at the petiole.

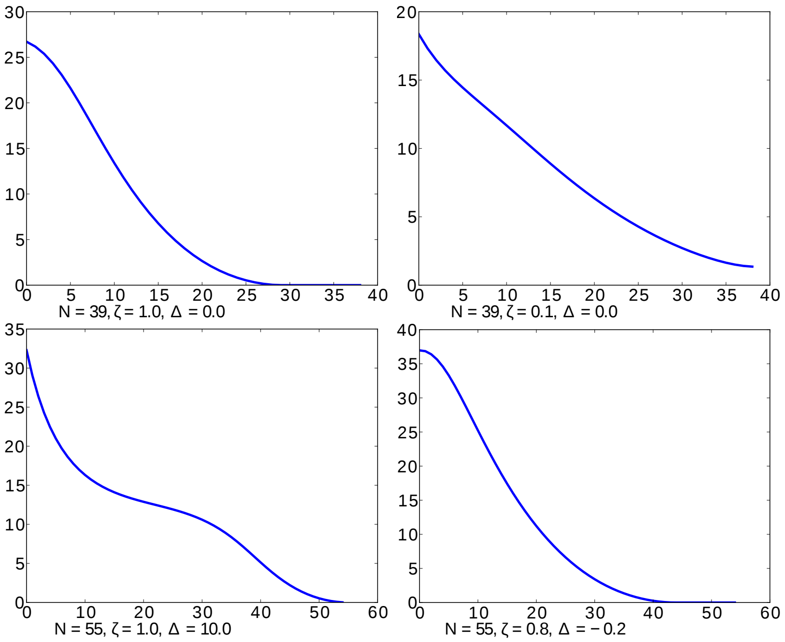


Figure 2: Optimal area distributions for the discrete numerical model using different parameter values. The $x$ axis corresponds to position along the needle, in contrast to the paper, $x = 0$ is the petiole. The $y$ axis shows total conductive area, non-normalized. Note that system length is not necessarily the whole needle. Additionally, none of the obtained shapes resemble the scaling law observed in real needles.

Numerical optimization was performed using the general purpose constrained nonlinear optimization algorithm IPOPT 3.11.x [3] together with Eric Xu's pyipopt[1].

Figure 2 shows the resulting area distributions for a set of parameter values. In contrast to the main paper, the petiole is at $x = 0$. It can be clearly seen that the optimal area distributions do not correspond to the scaling law seen in real needles and derived from power dissipation optimization.

Another possible optimizing function is $J_0/A_{01}$, the sugar flux at the petiole. In this case the optimizer will attempt to set $A_{01} = 0$, resulting in a singularity, i.e. there is no finite optimal solution in this case.

[1] `https://github.com/xuy/pyipopt`

### 2.3 Conclusion

We conclude that after analytical and numerical studies, sugar volume flow, sugar flux and thus energy flux are not relevant optimization quantities at the needle level, either because they cannot be optimized, or because the optima do not correspond to actual area distributions observed in real needles. In contrast, power dissipation optimization, as discussed in the main paper, provides a good explanation for the measured scaling laws in the phloem.

## References


[1] Kaare H Jensen, Kirstine Berg-Sø rensen, Søren M M Friis, and Tomas Bohr. Analytic solutions and universal properties of sugar loading models in Münch phloem flow. *Journal of Theoretical Biology*, 304:286–296, 2011.

[2] Kaare H Jensen and Maciej A Zwieniecki. Physical Limits to Leaf Size in Tall Trees. *Phys. Rev. Lett.*, 110(1):18104, January 2013.

[3] Andreas Wächter and Lorenz T. Biegler. On the implementation of an interior-point filter line-search algorithm for large-scale nonlinear programming. *Mathematical Programming*, 106(1):25–57, April 2005.
